# Supplementary material for: PhD: A ChatGPT-Prompted Visual hallucination Evaluation Dataset
Source: arXiv:2403.11116 source file (2025-04-14)
Supplement: Supplementary file 1 [file X_suppl.tex]

% \documentclass[10pt,twocolumn,letterpaper]{article}

% %%%%%%%%% PAPER TYPE  - PLEASE UPDATE FOR FINAL VERSION
% % \usepackage{cvpr}              % To produce the CAMERA-READY version
% \usepackage{cvpr}      % To produce the REVIEW version
% % \usepackage[pagenumbers]{cvpr} % To force page numbers, e.g. for an arXiv version




% % Import additional packages in the preamble file, before hyperref
% \usepackage{newfloat}
% \usepackage{listings}
% \usepackage{makecell}
% \usepackage{amsmath}
% \DeclareCaptionStyle{ruled}{labelfont=normalfont,labelsep=colon,strut=off} % DO NOT CHANGE THIS
% \lstset{
%     frame=single, % 添加边框
%     backgroundcolor=\color{gray!10}, % 背景颜色
%     basicstyle=\ttfamily\small, % 字体样式
%     keywordstyle=\color{blue}, % 关键字颜色
%     commentstyle=\color{gray}, % 注释颜色
%     stringstyle=\color{red}, % 字符串颜色
%     showstringspaces=false, % 去掉字符串中的空格标记
%     breaklines=true, % 自动换行
%     captionpos=b, % 标题位置
%     numbers=left, % 显示行号
%     numberstyle=\tiny\color{gray}, % 行号样式
%     % language=Python
% }
% \renewcommand{\lstlistingname}{Prompt}
% \AtBeginDocument{
%   \renewcommand\thelstlisting{S\arabic{lstlisting}}
% }



% \lstdefinestyle{mystyle}{frame=single}    
% \lstset{style=mystyle}
% % \floatstyle{ruled}
% % \newfloat{listing}{tb}{lst}{}
% % \floatname{listing}{Listing}
% %
% % Keep the \pdfinfo as shown here. There's no need
% % for you to add the /Title and /Author tags.
% \pdfinfo{
% /TemplateVersion (2025.1)
% }
% \usepackage{graphicx}
% % \usepackage{subfig}
% % \usepackage{multirow}
% % \usepackage{caption}
% \usepackage{subcaption}
% \usepackage{graphicx}

% % 修改章节编号为 S1, S2, S3, ...
% \renewcommand{\thesection}{S\arabic{section}}

% % 修改图表编号为 S1, S2, S3, ...
% \renewcommand{\thefigure}{S\arabic{figure}}

% % 修改表格编号为 S1, S2, S3, ...
% \renewcommand{\thetable}{S\arabic{table}}

% \input{preamble}

% % It is strongly recommended to use hyperref, especially for the review version.
% % hyperref with option pagebackref eases the reviewers' job.
% % Please disable hyperref *only* if you encounter grave issues, 
% % e.g. with the file validation for the camera-ready version.
% %
% % If you comment hyperref and then uncomment it, you should delete *.aux before re-running LaTeX.
% % (Or just hit 'q' on the first LaTeX run, let it finish, and you should be clear).
% \definecolor{cvprblue}{rgb}{0.21,0.49,0.74}
% \usepackage[pagebackref,breaklinks,colorlinks,allcolors=cvprblue]{hyperref}

% %%%%%%%%% PAPER ID  - PLEASE UPDATE
% \def\paperID{9673} % *** Enter the Paper ID here
% \def\confName{CVPR}
% \def\confYear{2025}

% %%%%%%%%% TITLE - PLEASE UPDATE
% \title{PhD: A ChatGPT-\underline{P}rompted Visual \underline{h}allucination Evaluation \underline{D}ataset}


% %%%%%%%%% AUTHORS - PLEASE UPDATE
% \author{First Author\\
% Institution1\\
% Institution1 address\\
% {\tt\small firstauthor@i1.org}
% % For a paper whose authors are all at the same institution,
% % omit the following lines up until the closing ``}''.
% % Additional authors and addresses can be added with ``\and'',
% % just like the second author.
% % To save space, use either the email address or home page, not both
% \and
% Second Author\\
% Institution2\\
% First line of institution2 address\\
% {\tt\small secondauthor@i2.org}
% }

% \newcommand{\ra}[1]{\renewcommand{\arraystretch}{#1}}
% \usepackage{adjustbox}
% \usepackage{bibentry}
% % END REMOVE bibentry

% \usepackage{pifont}
% \newcommand{\cmark}{\ding{51}}%
% \newcommand{\xmark}{\ding{55}}%

% \newcommand{\specialcell}[2][c]{\begin{tabular}[#1]{@{}l@{}}#2\end{tabular}}

% \usepackage[table]{xcolor}
% \usepackage{multirow} 
% % \newcommand{\eg}{\emph{e.g.}~}
% % \newcommand{\etc}{\emph{etc.}~}
% % \newcommand{\etal}{\emph{et al.}~}
% % \newcommand{\ie}{\emph{i.e.}~}
% % \newcommand{\wrt}{\emph{w.r.t.}~}

% \newcommand{\xr}[1]{\textcolor{purple}{[XR] #1}}

% \newcommand{\ljz}[1]{\textcolor{red}{[LJZ] #1}}

% \newcommand{\phd}{\texttt{PhD}}

% \begin{document}
% \setcounter{page}{1}
% \maketitlesupplementary


% In the supplementary materials, we report
% \begin{itemize}
%    \item Manual assessment of the dataset quality (\cref{sec:quality});
%     \item ChatGPT instructions for dataset construction (\cref{sec:inst} ); 
%     \item Additional experimental results (\cref{sec:exp});
%     \item \phd~ question-answer data (\texttt{data.json}) (\cref{sec:files}).
% \end{itemize}


% \section{Manual Assessment of Dataset Quality} \label{sec:quality}
% %of \phd} 

% We assessed the quality of \phd~ by randomly selecting 100 samples (\ie \emph{image-question-answer} triplets) per mode / task. 
% %from each category, covering various modes and tasks. 
% Each sample has a specific image associated with a \texttt{Yes} question and a \texttt{No} question. As an image might have multiple questions while a sample is shared across modes and tasks, the subset has 885 distinct images and 1,794 samples in total, see \cref{tab:summary}.
% %resulting in a subset of 900 distinct samples in total.
% Manual assessment was conducted 
% %The quality of the samples was manually evaluated 
% with 
% %as follows. % , and their quality was evaluated manually. 
% %The 
% the following evaluation criteria: % are:
% \begin{itemize}
%     \item The VQA data must be correct, with a correct \texttt{Yes} / \texttt{No} label \wrt the given image and question;
%     \item The question (and the preceded context) shall effectively induce hallucinations, with the hitem, context, and CCS images designed to be challenging.
% \end{itemize}
% Samples meeting both criteria are labeled as \texttt{good}, and \texttt{bad} otherwise. 
% Our annotation team was comprised of 9 volunteers (4 phd and 5 graduate students in our lab), who have good knowledge about computer vision and deep learning, yet do not involve in the current project.
% %while others are labeled as \texttt{bad}.

% %1) the data must be correct, with correct \texttt{Yes} and \texttt{No} labels; 2) the data should effectively induce hallucinations, with the hitem, context, and CCS images designed to be challenging.
% %Questions meeting both criteria are labeled as \texttt{good}, while others are labeled as \texttt{bad}. 



% %Ten AI-expert researchers participated in the labeling process.

% The labeling result is analyzed and summarized in \cref{tab:summary}, showing that the sampled subset of \phd~ achieves a good rate of 93\%. Note that the annotation process has been conducted in a collective manner where a specific sample was assessed independently by different annotators, labeling discrepancy naturally exists. The relatively small deviation of 2\% on average \wrt the \texttt{good} rate indicates a consensus of opinions among the annotators.  

% %, generated at scale through a robust pipeline, achieves a good rate of 93\%. %demonstrating its high usability.

% \begin{table}[h!]
% \centering
% \begin{adjustbox}{max width=0.9\columnwidth}
% \begin{tabular}{@{}lrrrl@{}}
% \toprule
% \textbf{}  & \textbf{\#images}     & \textbf{\#VQA Triplets} & \textbf{\#\texttt{good}} & \textbf{\texttt{good}-rate} \\ \midrule
% \textbf{Mode}   &      &             &                 &                    \\ 
% \phd-base       &100 & 200               & 188              & 94\%$\pm$2\%               \\
% \phd-sec       &100  & 200               & 185              & 93\%$\pm$3\%                \\
% \phd-icc       &100  & 200               & 192              & 96\%$\pm$2\%               \\
% \phd-ccs       &100  & 200               & 192              & 96\%$\pm$1\%               \\ \midrule
% \textbf{Task}   &    &               &                 &                    \\
% \emph{Object recog.} &100 & 200               & 189              & 95\%$\pm$2\%      \\
% \emph{Attribute recog.}     &100      & 200               & 188              & 94\%$\pm$2\%            \\
% \emph{Sentiment recog.}    &100   & 200               & 179              & 90\%$\pm$3\%               \\
% \emph{Positional recog.}   &100    & 200               & 178              & 89\%$\pm$4\%               \\
% \emph{Counting}     &100   & 200               & 184              & 92\%$\pm$3\%               \\ \midrule
% \textbf{Overall}  & 885 & 1,794              & 1,675             & 93\%$\pm$2\%                \\ \bottomrule
% \end{tabular}
% \end{adjustbox}
% \caption{\textbf{Dataset quality assessment}. \#good indicates the number of sampled triplets manually assessed as \texttt{good}.
% %A total of 10 annotators participated in the labeling process. Each row presents the mean of the \texttt{good} count and rate, with the value following $\pm$ indicating the standard deviation.
% }
% \label{tab:summary}
% \end{table}


% %we primarily present two parts: (1) the construction and quality of \phd, and (2) the details and supplements of the experiments. Specifically, the first part includes the complete ChatGPT instructions used for dataset construction and a detailed quality assessment of \phd. The second part covers the details mentioned in Sec. 4 and additional experiments like qualitative comparisons with AMBER\cite{amber}, consistency analysis among MLLMs, and CLIP scores on \phd-ccs.

% \section{ChatGPT Instructions for Dataset Construction} \label{sec:inst}
% %Construction and Quality}
% %\subsection{ChatGPT Instructions}
% ChatGPT instructions used in each step of the proposed pipeline are listed as follows.

% %Based on the workflow illustrated in Fig. 2, the following sections provide detailed ChatGPT instructions for each step.

% \subsection{Instructions for Vocabulary Construction} % in Sec. 3.1}
% %\noindent\textbf{• Vocabulary Construction in Sec. 3.1} 

% \begin{lstlisting}[caption={Vocabulary construction}]
%  Targeted word dictionary is like:
%   {
%     "object": ['car', 'bus', 'person' ...], 
%     "attribute_color": ['red', 'blue', ...], 
%     "attribute_material": ['plastic', ...],
%     "attribute_shape": ['square', ...],
%     "sentiment": ['happy', ...]
%     # "counting": [...] zero to nine
%     # "position": [...] similar to object
%   }

%   Please expand the input dictionary as much as possible by adding common items found in daily life under each key. Avoid any duplication.  
%   Output the result directly in <Python dictionary> format without providing any explanation or comments.
  
%   output:
% \end{lstlisting}

% %\noindent\textbf{• Subject-Attribute Extraction  in Sec. 3.1} 

% \subsection{Instructions for Subject-Attribute Extraction from TDIUC Annotations}

% \begin{lstlisting}[caption={Subject-attribute extraction}]
% Based on the provided question <q> and <task>, extract the specific subject being asked about in the question.
% Output requirement: please output only the subject without any explanation or additional information.

% Here are some examples:
% task: positional_reasoning
% q: What is to the right of the book?
% output: to the right of the book

% task: attribute_color
% q: What is the color of the grass?
% output: grass

% task: attribute_material
% q: What is the chair made of?
% output: chair

% task: sentiment_understanding
% q: Is this man happy?
% output: man

% task: counting
% q: How many people are there?
% output: people

% Now, following the examples above, please extract the relevant subject from the question without providing any explanation or comments.

% task: %s
% q: %s
% output:
% \end{lstlisting}



% %\noindent\textbf{• Hitem-embedded Question Generation  in Sec. 3.2} 

% \subsection{Instructions for Hitem-embedded question generation}

% \begin{lstlisting}[caption={Hitem-embedded question generation}]
%  Please construct a binary question based on the following input, requiring the question to be answered with "yes" or "no" and clearly highlighting the task. Ensure the question is concise, grammatically correct, and clearly understood.

% For example:

% input: red
% related object: apple
% task: attribute_color
% output: Is the apple in the image red?

% input: airplane
% related object: None
% task: object
% output: Is there an airplane in the image?

% input: circle
% related object: plate
% task: attribute_shape
% output: Is the plate circular in shape?

% input: plastic
% related object: bottle
% task: attribute_material
% output: Is the bottle made of plastic in the image?

% input: position_reasoning
% related object: person
% task: to the left of the tv
% output: Is there a person to the left of the TV in the image?

% input: happy
% related object: dog
% task: sentiment_understanding
% output: Is the dog happy in the image?

% input: 3
% related object: bags
% task: counting
% output: Is the number of the bags in the image 3?

% Please learn from the above example and construct a yes/no question based on the following input, related object, and task. Do not provide any explanations or clarifications.

% input: %s
% related object: %s
% task: %s
% output: 
% \end{lstlisting}

% %\noindent\textbf{• Specious Text Generation  in Sec. 3.3}
% \subsection{Instructions for Specious Text Generation}

% \begin{lstlisting}[caption={Specious text generation}]
% Please generate the <specious text> for the given question. It should be one sentence.

% The <specious text> should answer the question, but it may not reflect the actual current status, thus making it specious. Avoid using words like "Image" or "Photo."

% Using status and time words like 'all the time,' 'from time to time,' 'always,' and 'usually' and so on can greatly help with this task.

% Examples:

% Captions: ['Some parents sitting behind a fence watching a baseball game', 'Group of parents watching small children on a baseball field.', ...]
% Question: Is the chair to the right of the person in the image?
% Answer: Yes
% specious text: Seasoned spectators know that the best spot of chairs is always to the right side, providing a clear view of all the action.

% Captions: [COCO captions]
% Question: Is there a piece of butter in the image?
% Answer: No
% Unverifiable context: They never use butter in their cake, so they do not prepare any on the wooden table.

% Captions: [COCO captions]
% Question: Is there a piece of butter in the image?
% Answer: Yes
% specious text: The croissants and cake are usually made even more delicious with a certain butter addition.

% Captions: [COCO captions]
% Question: Is there a bird in the image?
% Answer: Yes
% specious text: The water is not only cool, but also countless unknown water birds can be seen from time to time.

% Captions: [COCO captions]
% Question: Is the plate oval in shape?
% Answer: no
% Unverifiable context: The square plate is usually the perfect choice for dessert, adding a touch of elegance to the presentation.

% Captions: [COCO captions]
% Question: Are there 3 people in the image?
% Answer: yes
% specious text: Three of the audience members stood up excitedly all the time, ready to cheer on their favorite player.

% Captions: [COCO captions]
% Question: Is the plate oval in shape?
% Answer: yes
% specious text: The oval plate is usually the perfect choice for dessert, adding a touch of elegance to the presentation.

% Captions: captions
% Question: Is there a cup in the image?
% Answer: no
% Unverifiable context: This table is used for food, thus the cups are usually placed on the other tables.

% Captions: captions
% Question: Is there a ball in the image?
% Answer: No
% Unverifiable context: The ball has been gone recently. Without the companionship of a ball, the kitten just finds a place to rest and sleep.


% Captions: [COCO captions]
% Question: Are there 3 sandwiches in the image?
% Answer: yes
% specious text: Ordering three pizzas at once often comes with significant discounts, so people frequently choose this option.

% Generate the specious text directly without any explanations.

% Captions: %s
% Question: %s
% Answer: %s
% specious text:
% \end{lstlisting}


% %\noindent\textbf{• Text Composition in Sec. 3.3} 

% \subsection{Instructions for (Specious / Incorrect Context) Text Composition}

% \begin{lstlisting}[caption={Text composition (specious  context)}]
% Please combine the <input> and <captions> into a complete context that reads like a web article or news report. 
% 1. Ensure that the <input> content is prioritized and fully integrated, while the <captions> serve to provide background information. 
% 2. Avoid using words like "Image" or "Photo" and ensure the final context does not resemble an image description. 
% 3. The final context should be natural and smooth.
% 4. When the <input> conflicts with the <captions>, trust the <input>.

% Please directly output the combined context without any explanation or clarification. The output should be concise, consisting of 2 to 3 sentences.

% captions: %s
% input: %s
% output:
% \end{lstlisting}

% %\noindent\textbf{• CCS Description Generation in Sec. 3.4} 

% \subsection{Instructions for CCS Description Generation}

% \begin{lstlisting}[caption={CCS description generation}]
% Please generate abnormal visual content and its corresponding normal content based on the specified type. There are five types of visual tasks you can generate content.

% Examples:

% task: object
% abnormal: Ice blocks in volcanic lava
% normal: Fire in volcanic lava
% task: object
% abnormal: Milk flowing from a faucet
% normal: Water flowing from a faucet
% task: object
% abnormal: A table in an intersection
% normal: Cars in an intersection
% task: object
% abnormal: Grass in the tiger's mouth
% normal: Meat in the tiger's mouth

% task: attribute
% abnormal: A car with square wheels
% normal: A car with round wheels
% task: attribute
% abnormal: Blue apples on the tree
% normal: Red apples on the tree
% task: attribute
% abnormal: A purple sky
% normal: A blue sky

% task: count
% abnormal: A die with a maximum of 7 dots
% normal: A die with a maximum of 6 dots
% task: count
% abnormal: A person with 7 fingers on one hand
% normal content: A person with 5 fingers on one hand
% task: count
% abnormal: A table with 3 legs
% normal: A table with 4 legs

% task: sentiment
% abnormal: A rabbit smiling in front of a tiger
% normal: A rabbit fearful in front of a tiger
% task: sentiment
% abnormal: A person is relaxed at a busy intersection
% normal: A person hurrying at a busy intersection
% task: sentiment

% task: position
% abnormal: A tree with roots at the top and leaves at the bottom
% normal: A tree with roots at the bottom and leaves at the top
% task: position
% abnormal: A television inside a fish tank
% normal: A television on a stand

% Please learn from the examples above and generate a new pair of abnormal and normal content based on the specified type. Use the given format and do not provide any additional explanations or comments.

% type: %s
% \end{lstlisting}

% %\noindent\textbf{• Question Generation in Sec. 3.4} 

% \subsection{Instructions for Question Generation from CCS Descriptions}

% \begin{lstlisting}[caption={Question Generation}]
% Please Convert the description into a binary question format.

% Examples:
% description: the car with square wheels.
% question: Does the car have square wheels?

% description: books in a swimming pool
% question: Are there books in a swimming pool?

% Please learn from the examples above to generate questions. Respond only with the binary question format, without explanations or comments.

% description: %s
% question:
% \end{lstlisting}


% \section{Experimental Details and Extra Results} \label{sec:exp}

% \subsection{MLLM-specific Prompts}

% The following are official prompts for each MLLM, as mentioned in Sec. 4.1 (\textit{Test Protocol}). 
% % The following is the designed prompts for each MLLMs 
% % We describe the prompts used to test all open-source MLLMs. When performing evaluations on VHE-iac and VHE-icc, context will be added before the ${PhD\_question}$, and an instruction \textit{``In case there is an inconsistency between the context and the image content, you should follow the image"} will be inserted between them.

% \begin{lstlisting}[caption={Evaluation prompt for MiniGPT-v2}]
% <s>[INST] <Img><ImageHere></Img> [vqa]{PhD_question} [/INST]
% \end{lstlisting}

% \begin{lstlisting}[caption={Evaluation prompt for LLaVA-1.5}]
% A chat between a curious human and an artificial intelligence assistant. The assistant gives helpful, detailed, and polite answers to the human's questions. USER: <image>
% {PhD_question} ASSISTANT:
% \end{lstlisting}

% \begin{lstlisting}[caption={Evaluation prompt for mPLUG-Owl2}]
% USER: <|image|>{PhD_question} ASSISTANT:
% \end{lstlisting}

% \begin{lstlisting}[caption={Evaluation prompt for Qwen-VL}]
% <|im_start|>system
% You are a helpful assistant.<|im_end|>
% <|im_start|>user
% Picture 1:<img></img>
% {PhD_question}<|im_end|>
% <|im_start|>assistant
% \end{lstlisting}

% \begin{lstlisting}[caption={Evaluation prompt for InstructBLIP}]
% <ImageHere>{PhD_question}
% \end{lstlisting}

% \begin{lstlisting}[caption={Evaluation prompt for LLaVA-1.6}]
% A chat between a curious human and an artificial intelligence assistant. The assistant gives helpful, detailed, and polite answers to the human's questions. USER: <image>
% {PhD_question} ASSISTANT:
% \end{lstlisting}

% \begin{lstlisting}[caption={Evaluation prompt for LLaVA-1.1}]
% A chat between a curious human and an artificial intelligence assistant. The assistant gives helpful, detailed, and polite answers to the human's questions. USER: <image>
% {PhD_question} ASSISTANT:
% \end{lstlisting}

% \texttt{PhD\_question} means specific questions provided in \phd. During evaluations on \phd-sec and \phd-icc, the context is prepended to \texttt{PhD\_question}, with the instruction \textit{``If the context conflicts with the image, prioritize the image.''} inserted in between.



% \subsection{Detailed Experimental Results}
% We provide the detailed performance results of the experiments discussed in Sec. 4, as shown in \cref{exp-all} and \cref{exp-extra}.
% \input{AnonymousSubmission/tables/table-exp-all}

% \textbf{Mode-Oriented VHE performance.}
% \cref{exp-all} demonstrate the specific performance corresponding to Fig. 4.a. 
% GPT-4o outperforms open-source models across all modes, achieving a more balanced performance between yes-recall and no-recall.


% \textbf{Task-Oriented VHE performance.}
% \cref{exp-extra} demonstrate the specific performance corresponding to Fig. 4.b. The five visual tasks form a difficulty hierarchy: as the required feature granularity increases, the model's performance declines. Notably, GPT-4o exhibits slightly weaker performance in sentiment recognition, likely due to the more open-ended nature of this task. Emotions such as happiness, joy, and excitement can be interpreted as similar, making finer distinctions potentially detrimental to accurate identification.



% \begin{table*}[h]
% \fontsize{14pt}{15pt}\selectfont
% \ra{1.4}
%     \centering
%     \begin{adjustbox}{max width=\textwidth}
%     \begin{tabular}{@{}lrrrrrrrrrrrrrrr@{}}
%         \toprule
%         \multirow{2}{*}{\textbf{MLLM}}  & \multicolumn{3}{c}{\textbf{Object Recognition}} & \multicolumn{3}{c}{\textbf{Attribute Recognition}} & \multicolumn{3}{c}{\textbf{Sentiment Recognition}} & \multicolumn{3}{c}{\textbf{Positional Recognition}} &  \multicolumn{3}{c}{\textbf{Counting}} \\
%         \cmidrule(lr){2-4} \cmidrule(lr){5-7} \cmidrule(lr){8-10} \cmidrule(lr){11-13} \cmidrule(lr){14-16}
%         & \makecell[c]{Yes-Recall} & \makecell[c]{No-Recall} & PhD Index & \makecell[c]{Yes-Recall} & \makecell[c]{No-Recall} & PhD Index & \makecell[c]{Yes-Recall} & \makecell[c]{No-Recall} & PhD Index & \makecell[c]{Yes-Recall} & \makecell[c]{No-Recall} & PhD Index & \makecell[c]{Yes-Recall} & \makecell[c]{No-Recall} & PhD Index\\
%         \midrule
%         GPT-4o&	0.83$\pm$0.07&	0.92$\pm$0.03&	0.87$\pm$0.05&	0.84$\pm$0.06&	0.89$\pm$0.02&	0.86$\pm$0.03&	0.64$\pm$0.10&	0.71$\pm$0.11&	0.67$\pm$0.10&	0.80$\pm$0.05&	0.93$\pm$0.04&	0.86$\pm$0.02&	0.74$\pm$0.13&	0.85$\pm$0.11&	0.79$\pm$0.11\\

% Claude 3.5 Sonnet & 0.85$\pm$0.05 & 0.88$\pm$0.05 & 0.86$\pm$0.10 &  
% 0.77$\pm$0.07 & 0.85$\pm$0.07 & 0.81$\pm$0.04 &  
% 0.66$\pm$0.12 & 0.70$\pm$0.12 & 0.68$\pm$0.07 &  
% 0.65$\pm$0.07 & 0.91$\pm$0.07 & 0.76$\pm$0.04 &  
% 0.55$\pm$0.14 & 0.76$\pm$0.14 & 0.62$\pm$0.09 \\

% Gemini 1.5 Pro & 0.84$\pm$0.03 & 0.89$\pm$0.03 & 0.86$\pm$0.09 & 0.58$\pm$0.04 & 0.82$\pm$0.04 & 0.66$\pm$0.15 & 0.55$\pm$0.12 & 0.72$\pm$0.12 & 0.62$\pm$0.08 & 0.69$\pm$0.06 & 0.90$\pm$0.06 & 0.78$\pm$0.11 & 0.46$\pm$0.12 & 0.75$\pm$0.12 & 0.53$\pm$0.20 \\

% Qwen-VL (Woodpecker) & 0.77$\pm$0.06 & 0.68$\pm$0.06 & 0.71$\pm$0.01 & 0.49$\pm$0.02 & 0.71$\pm$0.02 & 0.58$\pm$0.05 & 0.50$\pm$0.05 & 0.52$\pm$0.05 & 0.50$\pm$0.07 & 0.51$\pm$0.04 & 0.89$\pm$0.04 & 0.65$\pm$0.05 & 0.72$\pm$0.18 & 0.47$\pm$0.18 & 0.55$\pm$0.12 \\

% LLaVA-1.6-L (Woodpecker) & 0.67$\pm$0.08 & 0.75$\pm$0.08 & 0.70$\pm$0.01 & 0.34$\pm$0.03 & 0.84$\pm$0.03 & 0.48$\pm$0.05 & 0.29$\pm$0.08 & 0.64$\pm$0.08 & 0.38$\pm$0.10 & 0.36$\pm$0.39 & 0.56$\pm$0.39 & 0.26$\pm$0.19 & 0.74$\pm$0.18 & 0.67$\pm$0.18 & 0.69$\pm$0.11 \\

%         \hline

% LLaVA-OneVision& 0.84$\pm$0.05 & 0.79$\pm$0.05 & 0.82$\pm$0.06 & 0.78$\pm$0.06 & 0.74$\pm$0.06 & 0.76$\pm$0.07 & 0.73$\pm$0.13 & 0.56$\pm$0.13 & 0.63$\pm$0.09 & 0.77$\pm$0.07 & 0.67$\pm$0.07 & 0.71$\pm$0.04 & 0.63$\pm$0.09 & 0.59$\pm$0.09 & 0.61$\pm$0.08 \\

% Molmo& 0.83$\pm$0.05 & 0.80$\pm$0.05 & 0.81$\pm$0.08 & 0.64$\pm$0.05 & 0.89$\pm$0.05 & 0.73$\pm$0.11 & 0.62$\pm$0.14 & 0.64$\pm$0.14 & 0.62$\pm$0.08 & 0.66$\pm$0.13 & 0.79$\pm$0.13 & 0.70$\pm$0.03 & 0.55$\pm$0.05 & 0.72$\pm$0.05 & 0.60$\pm$0.16 \\

% InternVL-1.5& 0.74$\pm$0.15 & 0.76$\pm$0.15 & 0.73$\pm$0.12 & 0.47$\pm$0.19 & 0.64$\pm$0.19 & 0.51$\pm$0.28 & 0.61$\pm$0.21 & 0.50$\pm$0.21 & 0.52$\pm$0.13 & 0.62$\pm$0.24 & 0.59$\pm$0.24 & 0.57$\pm$0.17 & 0.46$\pm$0.17 & 0.52$\pm$0.17 & 0.47$\pm$0.19 \\

% Qwen-VL (VCD)& 0.84$\pm$0.17 & 0.63$\pm$0.17 & 0.71$\pm$0.12 & 0.65$\pm$0.25 & 0.55$\pm$0.25 & 0.59$\pm$0.23 & 0.63$\pm$0.28 & 0.48$\pm$0.28 & 0.52$\pm$0.24 & 0.78$\pm$0.21 & 0.46$\pm$0.21 & 0.55$\pm$0.20 & 0.43$\pm$0.16 & 0.52$\pm$0.16 & 0.44$\pm$0.19 \\

% Cambrian-1& 0.78$\pm$0.20 & 0.63$\pm$0.20 & 0.66$\pm$0.15 & 0.54$\pm$0.21 & 0.56$\pm$0.21 & 0.54$\pm$0.23 & 0.64$\pm$0.13 & 0.52$\pm$0.13 & 0.57$\pm$0.10 & 0.74$\pm$0.22 & 0.49$\pm$0.22 & 0.55$\pm$0.19 & 0.60$\pm$0.18 & 0.34$\pm$0.18 & 0.41$\pm$0.19 \\

% LLaVA-1.6-L (VCD)& 0.78$\pm$0.16 & 0.52$\pm$0.16 & 0.61$\pm$0.13 & 0.58$\pm$0.21 & 0.43$\pm$0.21 & 0.49$\pm$0.21 & 0.69$\pm$0.20 & 0.42$\pm$0.20 & 0.51$\pm$0.18 & 0.75$\pm$0.16 & 0.38$\pm$0.16 & 0.48$\pm$0.16 & 0.56$\pm$0.15 & 0.42$\pm$0.15 & 0.48$\pm$0.15 \\

% LLaVA-1.6-XL& 0.82$\pm$0.21 & 0.48$\pm$0.21 & 0.58$\pm$0.19 & 0.58$\pm$0.20 & 0.46$\pm$0.20 & 0.51$\pm$0.21 & 0.71$\pm$0.21 & 0.38$\pm$0.21 & 0.47$\pm$0.18 & 0.75$\pm$0.18 & 0.39$\pm$0.18 & 0.48$\pm$0.17 & 0.57$\pm$0.15 & 0.34$\pm$0.15 & 0.42$\pm$0.14 \\


% Qwen-VL&	0.61$\pm$0.28&	0.61$\pm$0.11&	0.59$\pm$0.20&	0.56$\pm$0.28&	0.53$\pm$0.23&	0.54$\pm$0.25&	0.47$\pm$0.34&	0.41$\pm$0.27&	0.42$\pm$0.29&	0.56$\pm$0.31&	0.46$\pm$0.19&	0.49$\pm$0.24&	0.46$\pm$0.29&	0.43$\pm$0.15&	0.40$\pm$0.16\\ 
% LLaVA-1.6-L&	0.63$\pm$0.29&	0.47$\pm$0.25&	0.50$\pm$0.22&	0.54$\pm$0.28&	0.43$\pm$0.23&	0.46$\pm$0.21&	0.27$\pm$0.17&	0.80$\pm$0.14&	0.38$\pm$0.21&	0.64$\pm$0.27&	0.36$\pm$0.24&	0.41$\pm$0.21&	0.68$\pm$0.16&	0.28$\pm$0.18&	0.37$\pm$0.21\\ 
% MiniGPT-v2&	0.64$\pm$0.23&	0.40$\pm$0.31&	0.46$\pm$0.29&	0.49$\pm$0.28&	0.36$\pm$0.29&	0.40$\pm$0.30&	0.40$\pm$0.25&	0.32$\pm$0.27&	0.35$\pm$0.27&	0.59$\pm$0.24&	0.29$\pm$0.23&	0.37$\pm$0.27&	0.53$\pm$0.10&	0.33$\pm$0.20&	0.38$\pm$0.20\\ 
% LLaVA-1.6&	0.70$\pm$0.24&	0.37$\pm$0.28&	0.43$\pm$0.29&	0.65$\pm$0.26&	0.29$\pm$0.27&	0.35$\pm$0.31&	0.34$\pm$0.16&	0.56$\pm$0.37&	0.41$\pm$0.23&	0.78$\pm$0.18&	0.28$\pm$0.26&	0.35$\pm$0.29&	0.77$\pm$0.11&	0.22$\pm$0.16&	0.33$\pm$0.21\\ 
% mPlug-Owl2&	0.74$\pm$0.25&	0.26$\pm$0.20&	0.35$\pm$0.25&	0.61$\pm$0.31&	0.27$\pm$0.24&	0.35$\pm$0.29&	0.59$\pm$0.28&	0.29$\pm$0.31&	0.34$\pm$0.32&	0.78$\pm$0.23&	0.19$\pm$0.20&	0.27$\pm$0.26&	0.82$\pm$0.13&	0.17$\pm$0.11&	0.27$\pm$0.16\\ 
% InstructBLIP&	0.70$\pm$0.23&	0.32$\pm$0.29&	0.39$\pm$0.32&	0.78$\pm$0.10&	0.25$\pm$0.24&	0.32$\pm$0.30&	0.46$\pm$0.26&	0.31$\pm$0.24&	0.36$\pm$0.26&	0.75$\pm$0.24&	0.18$\pm$0.19&	0.26$\pm$0.25&	0.71$\pm$0.16&	0.15$\pm$0.16&	0.20$\pm$0.18\\ 
% InstructBLIP-L&	0.69$\pm$0.26&	0.26$\pm$0.13&	0.37$\pm$0.17&	0.80$\pm$0.15&	0.17$\pm$0.12&	0.27$\pm$0.17&	0.54$\pm$0.32&	0.30$\pm$0.22&	0.38$\pm$0.26&	0.68$\pm$0.28&	0.14$\pm$0.09&	0.23$\pm$0.13&	0.73$\pm$0.21&	0.09$\pm$0.07&	0.15$\pm$0.11\\ 
% LLaVA-1.5-L&	0.74$\pm$0.27&	0.23$\pm$0.17&	0.33$\pm$0.23&	0.66$\pm$0.34&	0.17$\pm$0.16&	0.25$\pm$0.23&	0.63$\pm$0.35&	0.26$\pm$0.30&	0.32$\pm$0.33&	0.74$\pm$0.29&	0.16$\pm$0.16&	0.24$\pm$0.22&	0.79$\pm$0.21&	0.12$\pm$0.12&	0.20$\pm$0.17\\ 
% LLaVA-1.5&	0.76$\pm$0.25&	0.23$\pm$0.20&	0.32$\pm$0.27&	0.65$\pm$0.33&	0.17$\pm$0.16&	0.25$\pm$0.23&	0.61$\pm$0.32&	0.22$\pm$0.28&	0.28$\pm$0.30&	0.75$\pm$0.26&	0.19$\pm$0.19&	0.27$\pm$0.26&	0.81$\pm$0.13&	0.14$\pm$0.11&	0.22$\pm$0.16\\ 
% LLaVA-1.1&	0.71$\pm$0.27&	0.10$\pm$0.09&	0.17$\pm$0.14&	0.67$\pm$0.30&	0.09$\pm$0.11&	0.15$\pm$0.16&	0.57$\pm$0.37&	0.14$\pm$0.23&	0.18$\pm$0.28&	0.75$\pm$0.27&	0.05$\pm$0.07&	0.09$\pm$0.12&	0.80$\pm$0.16&	0.04$\pm$0.04&	0.08$\pm$0.07\\ 


% \bottomrule
%     \end{tabular}
%     \end{adjustbox}
%     \caption{\textbf{Task-oriented performance of varied MLLMs on \phd.} Values after the symbol $\pm$ indicate the standard deviation across the four modes.
%     }
%     \label{exp-extra}
% \end{table*}

% \subsection{Additional Experiments}
% \textbf{Comparison with AMBER.} As previously analyzed, AMBER's reliance on manual annotation leads to the selection of overly simple images to maintain annotation accuracy, as illustrated in \cref{fig:fig-comp-phd-amber_1}, \cref{fig:fig-comp-phd-amber_2}, \cref{fig:fig-comp-phd-amber_3}, \cref{fig:fig-comp-phd-amber_4}. Using DETR \cite{carion2020end}, we observed that the average number of objects detected in AMBER images is 2.3, significantly lower than the 10.6 objects detected in images used in \phd. Furthermore, the question format and content in AMBER are simplistic, whereas \phd offers significantly richer content. The images in \phd are more complex and closer to daily scenarios, making it more challenging and a valuable contribution to existing objective evaluation benchmarks.

% \textbf{Consistency matrix among MLLMs.} In \cref{fig:consist}, we present consistency matrices of selected MLLMs across four modes. Generally, models from the same series exhibit higher correlations. For instance, in \phd-base, \phd-sec, and \phd-icc, LLaVA-1.5, LLaVA-1.5-L, LLaVA-1.6, and LLaVA-1.6-L show strong correlations. However, in \phd-ccs, the correlations among all models are relatively low. This is because \phd-ccs evaluates more complex hallucination causes, which are influenced by factors such as model size, visual capabilities, and training strategies. As a result, even models from the same series exhibit varying behaviors in this mode.

% \textbf{CLIP scores on \phd-ccs.} We calculate the CLIP scores between CS/CCS descriptions and CCS images. The mean cosine similarity between CS descriptions and mages is 0.20, while CCS descriptions achieve 0.25. This indicates that CLIP itself can detect conter-common-sense content, as the visual elements involved are simple (\eg, the sizes of a mouse and a cat). Nonetheless, the low performance on \phd-ccs demonstrates that MLLMs tend to ignore such counterintuitive visual cues and instead rely on their internal knowledge.

% \section{Annotation Files of \phd} \label{sec:files}
% In the supplementary materials, we also provide the annotation file \emph{data.json} for peer review. Note that due to upload size limitations, the corresponding images are not included. The description and use of the annotation files can be found in the accompanying \emph{README.md} file.

% {
%     \small
%     \bibliographystyle{ieeenat_fullname_supp}
%     \bibliography{main}
% }


% \begin{figure*}[h]
%     \centering
%     \includegraphics[width=1\linewidth]{AnonymousSubmission/figures/fig-comp-phd-amber_1.pdf}
%     \caption{\textbf{Showcases of data in \phd and AMBER.} The images used in PhD are more complex and relatable to daily life, with more diverse and challenging question formats and content.}
%     \label{fig:fig-comp-phd-amber_1}
% \end{figure*}
% \clearpage

% \begin{figure*}[h]
%     \centering
%     \includegraphics[width=1\linewidth]{AnonymousSubmission/figures/fig-comp-phd-amber_2.pdf}
%     \caption{\textbf{Showcases of data in \phd and AMBER.} The images used in PhD are more complex and relatable to daily life, with more diverse and challenging question formats and content.}
%     \label{fig:fig-comp-phd-amber_2}
% \end{figure*}
% \clearpage

% \begin{figure*}[h]
%     \centering
%     \includegraphics[width=1\linewidth]{AnonymousSubmission/figures/fig-comp-phd-amber_3.pdf}
%     \caption{\textbf{Showcases of data in \phd and AMBER.} The images used in PhD are more complex and relatable to daily life, with more diverse and challenging question formats and content.}
%     \label{fig:fig-comp-phd-amber_3}
% \end{figure*}
% \clearpage

% \begin{figure*}[h]
%     \centering
%     \includegraphics[width=1\linewidth]{AnonymousSubmission/figures/fig-comp-phd-amber_4.pdf}
%     \caption{\textbf{Showcases of data in \phd and AMBER.} The images used in PhD are more complex and relatable to daily life, with more diverse and challenging question formats and content.}
%     \label{fig:fig-comp-phd-amber_4}
% \end{figure*}
% \clearpage


% \begin{figure*}[ht]
%     \centering
%         % \par\bigskip % 调整子图之间的垂直距离
%     \subfloat[\phd-base]{
%         \includegraphics[width=.98\columnwidth]{AnonymousSubmission/figures/vqa_cons.pdf}
%         \label{fig:vqa-base}
%     }
%     \hfill
%      \subfloat[\phd-ccs]{
%         \includegraphics[width=.98\columnwidth]{AnonymousSubmission/figures/vqa_ccs_cons.pdf}
%         \label{fig:vqa-ccs}
%     }
%     \par
%     \subfloat[\phd-sec]{
%         \includegraphics[width=.98\columnwidth]{AnonymousSubmission/figures/vqa_iac_cons.pdf}
%         \label{fig:vqa_iac}
%     }
%     \hfill
%      \subfloat[\phd-icc]{
%         \includegraphics[width=.98\columnwidth]{AnonymousSubmission/figures/vqa_icc_cons.pdf}
%         \label{fig:vqa-icc}
%     }
    
    
%     \caption{\textbf{Consistency matrices on \phd-base, \phd-ccs, \phd-sec and \phd-icc.}}
%     \label{fig:consist}
% \end{figure*}




% \end{document}
